# Supplementary material for: Anisotropic intrinsic lattice thermal conductivity of phosphorene from first principles
Source: arXiv:1409.0279 source file (2015-02-05)
Supplement: Supplementary file 1 [file Supplemental_Material.pdf]

# Supplemental Material

## Anisotropic intrinsic lattice thermal conductivity of phosphorene from first principles

Guangzhao Qin[a], Qing-Bo Yan[*a], Zhenzhen Qin[b], Sheng-Ying Yue[‡c], Ming Hu[*d,e] and Gang Su[*c]

[a] College of Materials Science and Opto-Electronic Technology, University of Chinese Academy of Sciences, Beijing 100049, China. E-mail: *yan@ucas.ac.cn*

[b] College of Electronic Information and Optical Engineering, Nankai University, Tianjin 300071, China.

[c] School of Physics, University of Chinese Academy of Sciences, Beijing 100049, China. E-mail: *gsu@ucas.ac.c*n

[d] Institute of Mineral Engineering, Division of Materials Science and Engineering, Faculty of Georesources and Materials Engineering, RWTH Aachen University, Aachen 52064, Germany. E-mail: *hum@ghi.rwth-aachen.de*

[e] Aachen Institute for Advanced Study in Computational Engineering Science (AICES), RWTH Aachen University, Aachen 52062, Germany.

[‡] Present address: Aachen Institute for Advanced Study in Computational Engineering Science (AICES), RWTH Aachen University, Aachen 52062, Germany.

# 1. Details on the workflow

The workflow and equations for calculating the thermal conductivity are described in the references related to the ShengBTE code [1,2]. For example, the thermal conductivity could be obtained based on the equation:

$$\kappa_l^{\alpha\beta} = \frac{1}{k_B T^2 \Omega N} \sum_\lambda f_0(f_0+1)(\hbar\omega_\lambda)^2 v_\lambda^\alpha F_\lambda^\beta ,$$

where $\Omega$ is the volume of the unit cell, $f_0$ is the zero-order term of the phonon distribution function, $\lambda$ is the index of phonon mode comprising both phonon branch index and wave vector, $\omega$ is the angular frequency, $v$ is the group velocity, $F_\lambda$ is defined based on the expansion of phonon distribution assuming the small enough $\nabla T$:

$$f_\lambda = f_0(\omega_\lambda) - F_\lambda \bullet \nabla T \frac{df_0}{dT} ,$$

and when only considering the scattering mechanism of two- and three-phonon processes, $F_\lambda$ could be calculated with the formula:

$$F_\lambda = \tau_\lambda^0 (v_\lambda + \Delta_\lambda) ,$$

where $\tau_\lambda^0$ is the relaxation time obtained from perturbation theory:

$$\frac{1}{\tau_\lambda^0} = \frac{1}{N} \left( \sum_{\lambda'\lambda''}^{+} \Gamma_{\lambda\lambda'\lambda''}^{+} + \sum_{\lambda'\lambda''}^{-} \frac{1}{2} \Gamma_{\lambda\lambda'\lambda''}^{-} + \sum_{\lambda'} \Gamma_{\lambda\lambda'} \right) ,$$

where $\Gamma_{\lambda\lambda'\lambda''}^{+}$ and $\Gamma_{\lambda\lambda'\lambda''}^{-}$ are three-phonon scattering rates corresponding to absorption and emission processes of phonon, respectively, and $\Gamma_{\lambda\lambda'}$ is the scattering possibility from isotopic disorder.

## 2. The supercell size for phonon calculations

In order to determine the supercell size used in the DFPT calculations and the subsequent calculations of the 3-rd IFCs, we performed calculations with the supercell size of 1x1x1, 2x2x1, 3x3x1, 4x4x1 and 5x5x1. The corresponding phonon dispersion curves show a convergence as the supercell size increasing, such as the coupling between optical and acoustic phonon branches, the smoothness of the phonon dispersion curves and the shift of frequencies of each mode. Since there is no difference between the results obtained with the supercell size of 4x4x1 and 5x5x1, it is doubtless that the supercell size of 5x5x1 is a good choice.

## 3. The vibration of phonon modes

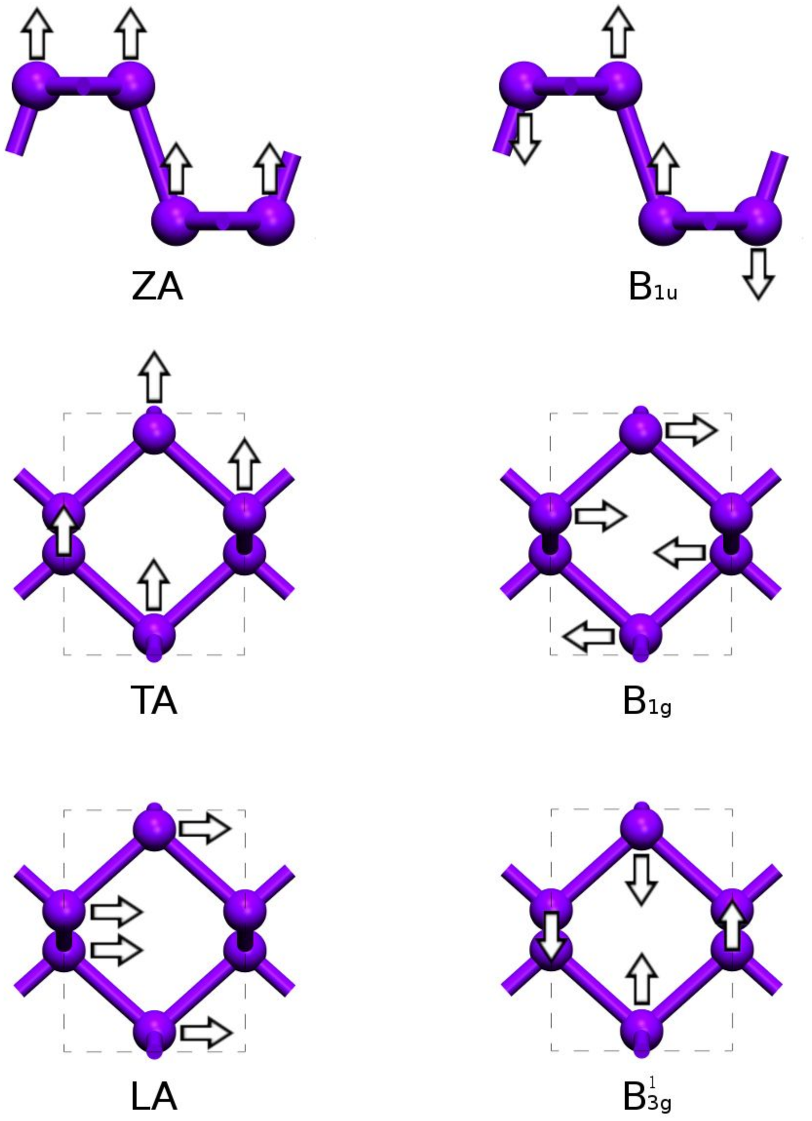


Considering the very long relaxation time of the optical phonon branch $B_{1g}$, the $B_{1g}$ mode contributes much more than other optical phonon branches to the thermal conductivity. The very long relaxation time of the $B_{1g}$ mode might lie in the same vibrational direction (zigzag) of the $B_{1g}$ mode as the acoustic phonon branch LA, which also possesses a relative long relaxation time. Thus the zigzag direction is the most favorable direction for phonon thermal transport due to the less scattering.

# 4. Born effective charge

Table S I. Born effective charge tensors obtained based on DFPT.

| Atom | Born effective charge (*Z**) | | | | | | | | |
|---|---|---|---|---|---|---|---|---|---|
| | $Z_{xx}$ | $Z_{xy}$ | $Z_{xz}$ | $Z_{yx}$ | $Z_{yy}$ | $Z_{yz}$ | $Z_{zx}$ | $Z_{zy}$ | $Z_{zz}$ |
| $P_1$ | -0.00065 | -0.00100 | 0.00082 | 0.00000 | 0.01180 | 0.45136 | 0.00000 | 0.01892 | 0.00435 |
| $P_2$ | -0.00065 | 0.00100 | -0.00082 | 0.00000 | 0.00951 | 0.45463 | 0.00000 | 0.01916 | 0.00396 |
| $P_3$ | -0.00065 | -0.00100 | -0.00082 | 0.00000 | 0.01180 | -0.45136 | 0.00000 | -0.01916 | 0.00396 |
| $P_4$ | -0.00065 | 0.00100 | 0.00082 | 0.00000 | 0.00951 | -0.45463 | 0.00000 | -0.01892 | 0.00435 |

# References


[1] W. Li, L. Lindsay, D. A. Broido, D. A. Stewart and N. Mingo, *Phys. Rev. B*, 2012, **86,** 174307.

[2] W. Li, J. Carrete, N. A. Katcho and N. Mingo, *Comput. Phys. Commun.*, 2014, **185,** 1747-1758.
